# Supplementary material for: Effect of magnetic and non-magnetic impurities on the spin dimers in the spin 1/2 chains of quantum magnet Sr$_{14}$Cu$_{24}$O$_{41}$
Source: arXiv:1808.00830 source file (2018-08-02)
Supplement: Supplementary file 1 [file Supplementary_Information_Bag_et_al..pdf]

# Supplementary Information on

## Effect of magnetic and non-magnetic impurities on the spin dimerizations in the spin 1/2 chains of $Sr_{14}Cu_{24}O_{41}$


**Rabindranath Bag[1], Koushik Karmakar[1], Sudesh Dhar[2], Malvika Tripathi[3], R. J. Choudhary[3], and Surjeet Singh[1,4*]**

[1]Indian Institute of Science Education and Research, Dr. Homi Bhabha Road, Pune, Maharashtra-411008, India

[2]Tata Institute of Fundamental Research, Mumbai, Maharashtra, India

[3]UGC DAE Consortium for Scientific Research, Indore 452001, India

[4]Centre for Energy Science, Indian Institute of Science Education and Research,

Dr. Homi Bhabha Road, Pune, Maharashtra-411008, India


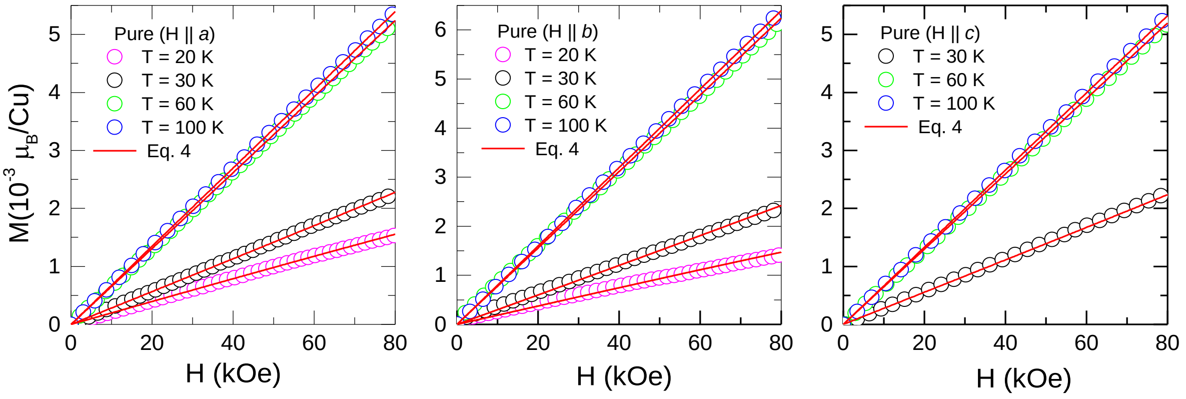


**Figure S1**: Isothermal magnetization data (MH) of a pristine $Sr_{14}Cu_{24}O_{41}$ crystal for various temperatures above T = 10 K. The data are fitted by using the equation (1) in the text. The value of $N_D^{ZR}$ and $J_{ZR}$ were fixed from the value obtained from the $\chi$(T) fitting in the main text. The parameter $N_s$ is treated as free and the best-fit values of $N_s$ at various temperatures are tabulated below.

$$\boldsymbol{M(H) = \chi_0 H + N_s N_A g\mu_B B_{1/2}(g\mu_B H/2k_BT) + 2N_d^{ZR} N_A g\mu_B\left[sinh(g\mu_B H/2k_BT)/\{1 + e^{J_{ZR}/k_BT} + 2cosh(g\mu_B H/2k_BT)\}\right]} \quad \textbf{(1)}$$

**Table I**: The value of the fitting parameter $N_S$ (no. of free spins per Cu) obtained using Eq. 4 corresponding to Fig. S1:

| Temperature | H \|\| a | H \|\| b | H \|\| c |
|---|---|---|---|
| T = 20 K | 0.0063(2) | -- | -- |
| T = 30 K | 0.0068(2) | 0.007(1) | 0.0063(2) |
| T = 60 K | 0.0072(2) | 0.010(1) | 0.0065(2) |
| T = 100 K | 0.0085(2) | 0.013(1) | 0.0069(2) |

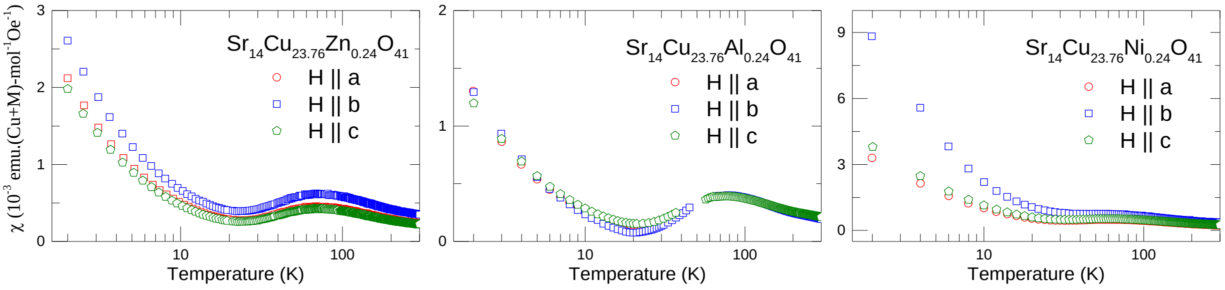


**Figure S2**: Temperature variation of magnetic susceptibility c of 1% Zn, Al and Ni doped $Sr_{14}Cu_{24}O_{41}$ single crystals.

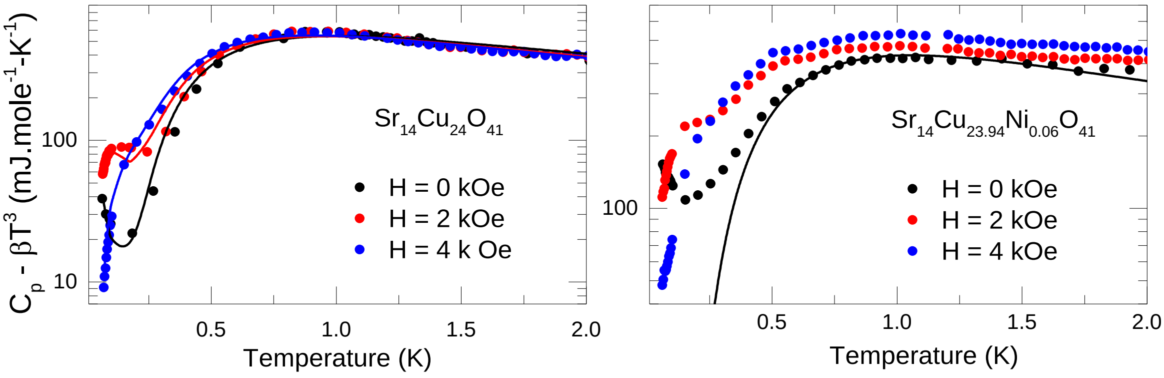


**Figure S3**: The low temperature specific heat ($C_p$) of an undoped and a 0.25% Ni doped $Sr_{14}Cu_{24}O_{41}$ single crystals measured under H = 0, 2 and 4 kOe. The phononic contribution, which is small in this temperature range, is subtracted from $C_p$. Solid lines are fit to the data. The fitting procedure and the associated fitting parameters are described in the text.

**Specific heat fitting procedure:**

We first estimated the specific heat due to lattice vibrations by approximating the total measured specific heat in the temperature range 10 K to 15 K as $C_p \sim C_{ph} = \beta T^3$, which fitted the data fairly nicely. The subtracted data below T = 2 K consists of: (1) the Schottky contribution ($C_{Sch}$) due to a small number of spins that remain undimerized down to the lowest temperature, and (2) the dimer contribution ($C_{dimer}$) arising from the long-distance dimers. Due to variable length of these dimers, the exchange $J_{LD}$ is expected to have a

narrow distribution of values -narrow because $x_{Ni}$ is very small. Here, we approximate the distribution by a single value $J_{LD} = \Delta$.

The expression for the low-temperature specific heat, therefore, takes the form: $C_p - \beta T^3 = C_{Sch} + C_{dimer\,(\Delta_1)} + C_{dimer}(\Delta_2)$, where $C_{Sch} = N_f R(2\mu_B/k_B T)^2 \frac{exp(-2\mu_B H/k_B T)}{[1+exp(-2\mu_B/k_B T)]^2}$ , and $C_{dimer}(\Delta) = A\left(\frac{\Delta}{T}\right)^{3/2} exp\left(\frac{\Delta}{T}\right)$.

In these expressions symbols have their usual meanings. The coefficient A of the dimer term is proportional to the number of long-distance dimers $N_D^{LD}$. The fitting results are shown in Figure S3, and the values of the fitting parameters are collected in the table II below:

**Table II:** Values of the fitting parameters corresponding to Fig. S3

| Specimen | H (Oe) | $H_{cal}$ (Oe) | $N_f$ /f.u. | A /f.u. | Δ (K) |
|---|---|---|---|---|---|
| Undoped (0.06 to 2 K) | 0 | 439 | 0.029 | 1330 | 1.50 |
| | 2000 | 1874 | 0.023 | 1319 | 1.42 |
| | 4000 | 3383 | 0.020 | 1319 | 1.38 |
| Ni 0.25 % (0.50 to 2 K) | 0 | -- | -- | 1056 | 1.58 |

In order to fit the data for the Ni-doped crystal below T = 0.5 K, we should consider not only the Schottky term due to S = 1/2 but also due to S = 1 (Ni spins), which make the fitting procedure more cumbersome with larger number of free parameters. Since in the present paper, our interest is mainly pertains to the anomaly associated with the long-distance dimers, we fitted the data above T = 0.5 K using the dimer term alone. It should be noted that this procedure, may not work in the presence of a magnetic field since a substantial weight of the low-temperature Schottky term shifts to higher temperatures in the presence of an applied magnetic field.

From the table above one can quantify the effect of Ni doping on the long-distance dimer. From the fitting of the zero-field data, we find ΔA (%) = 21 %. **This suggest that 21 % of LDDs will be severed in the presence of Ni impurity.**

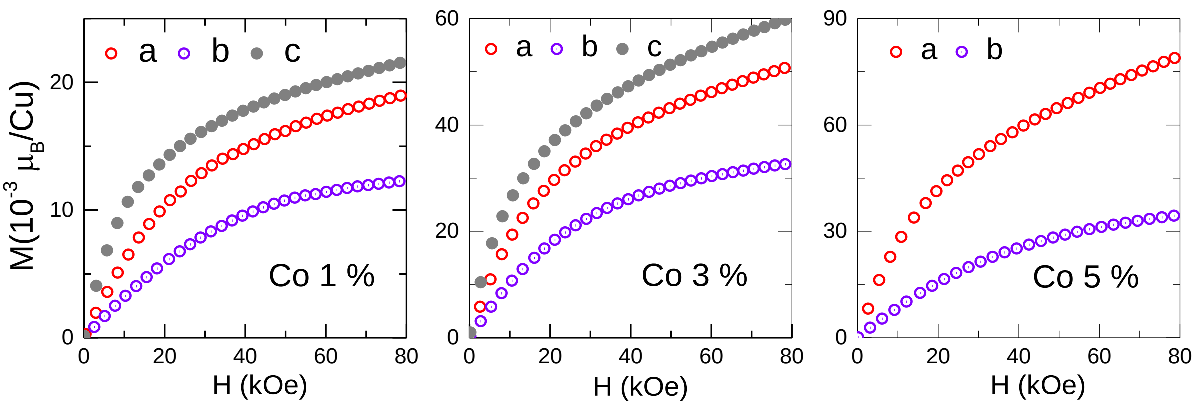


**Figure S5**: Isothermal magnetization at T = 2 K for Co 1, 3 and 5 % crystals.
